# Supplementary material for: Structural and electronic transformations in TiO2 induced by electric current
Source: arXiv:2409.08223 ancillary file (2024-10-21)
Supplement: Supplementary file 1 [file supp.pdf]

# Supplementary material for “Structural and electronic transformations in $\text{TiO}_2$ induced by electric current”

*Tyler C. Sterling<sup>‡</sup>, Feng Ye<sup>2</sup>, Seohyeon Jo<sup>3</sup>, Anish Parulekar<sup>1</sup>, Yu Zhang<sup>1</sup>,  
Gang Cao<sup>1,4</sup>, Rishi Raj<sup>5</sup>, and Dmitry Reznik<sup>1,4</sup>*

<sup>1</sup> *Department of Physics, University of Colorado Boulder, Boulder, CO, 80309, USA*

<sup>2</sup> *Neutron Scattering Division, Oak Ridge National Lab, Oak Ridge, TN, 37830, USA*

<sup>3</sup> *Materials Science and Engineering, University of Colorado Boulder, Boulder, CO, 80309, USA*

<sup>4</sup> *Department of Mechanical Engineering, University of Colorado Boulder, Boulder, CO, 80309, USA*

<sup>5</sup> *Center for Experiments on Quantum Materials, University of Colorado Boulder, Boulder, CO, 80309, USA*

## 1 Determining the needle directions

The directions of the diffuse scattering “needles” are determined by fitting the coordinates of the intersection of the needles with integrated planes of intensity cut through the data. To improve statistics and remove the effects of structure factor on the intensity, we summed the data in all Brillouin zones with diffuse features into a single Brillouin zone. The fits are done using the intensity in the summed data sets.

The original orientations of the needles were determined by fitting the intersections through planes perpendicular to the reciprocal lattice vectors of the crystal. These coordinates were used to construct projection vectors  $\mathbf{u}$ ,  $\mathbf{v}$ , and  $\mathbf{w}$ , one set for each needle. The vectors are calculated in Cartesian coordinates with each vector having unit length, e.g.  $|\mathbf{u}| = 1 \text{ \AA}^{-1}$ . The vectors are chosen as follows: (i)  $\mathbf{u}$  points along the needle and is found by fitting the intensity in cuts through the needle. (ii)  $\mathbf{v}$  is chosen perpendicular to the plane containing the  $\mathbf{u}$  vector of interest and a  $\mathbf{u}$  vector belonging to a different needle.  $\mathbf{w}$  is chosen as  $\mathbf{w} = \mathbf{u} \times \mathbf{v}$ . A set of projection vectors is shown in fig. S1. In the basis of a

---

<sup>‡</sup>ty.sterling@colorado.edu

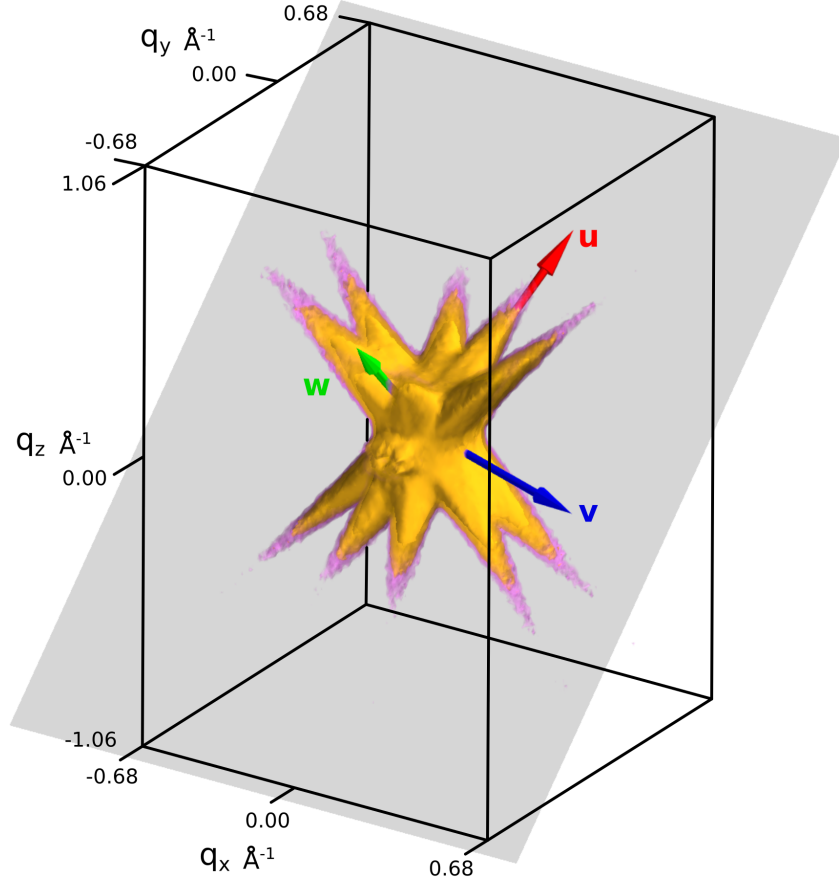

Fig. 1: Projection vectors  $\mathbf{u}$ ,  $\mathbf{v}$ , and  $\mathbf{w}$  plotted with the summed S1 data set.  $\mathbf{u}$  is parallel to the needle it is plotted on.  $\mathbf{v}$  is in the plane containing two symmetry equivalent  $\mathbf{u}$ .  $\mathbf{w}$  is parallel to  $\mathbf{u} \times \mathbf{v}$ .

given needle, we specify coordinates  $\mathbf{q} = \xi\mathbf{u} + \eta\mathbf{v} + \zeta\mathbf{w}$  where  $\xi$ ,  $\eta$ , and  $\zeta$  are the distance along  $\mathbf{u}$ ,  $\mathbf{v}$ , and  $\mathbf{w}$  respectively.

Since the needles intersect planes perpendicular to the reciprocal lattice vectors at angles, the original integrated intensities are asymmetric, introducing error into the fits. To improve the fits, the original projections are used to integrate the data in planes that are approximately perpendicular to the needles. Planes are integrated in steps along each  $\mathbf{u}$  vector and the coordinates of the needle are fit at each step. Examples of data integrated using the final projections are shown in fig. S2 (a) and (c). In some cases, other needles than the one of interest in a given plane intersects near the origin too (see fig. S2 (a)-(d)). To account for the other needles in a given plane, all of the needles intersecting each plane are fit simultaneously. The center, widths, and orientations of the intersections are denoted by the lines in fig. S2 (b) and (d). The bold, unbroken lines correspond to the needle position of interest in each plane. The needle directions are all equivalent under tetragonal symmetry operations: the reported direction for each data set is determined by averaging the fits over all steps and over all needles.

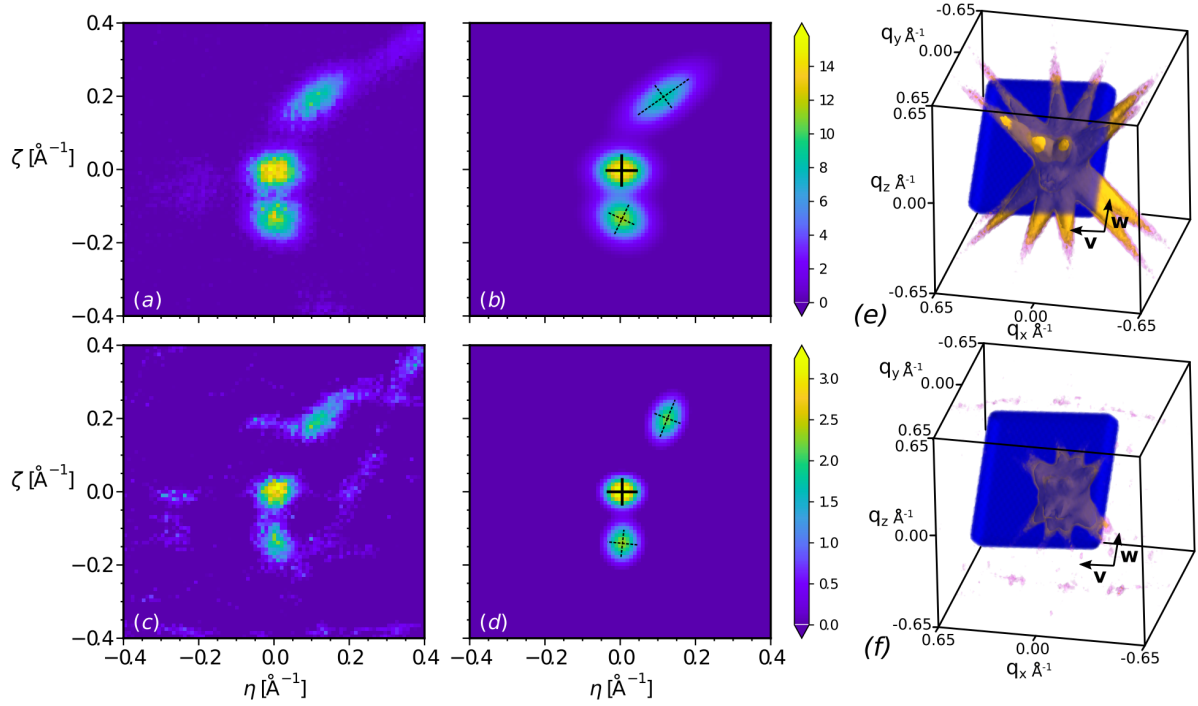

Fig. 2: Fits to the needle directions in the S1 ((a),(b),(e)) and in-situ 100C, 500 mA ((c),(d),(f)) data sets. (a) Integrated data in the region shown in (e) taken from the summed S1 data set. (b) Fit to the data in (a). The coordinate of the intersection of the needle is  $\mathbf{q} = \xi\mathbf{u} + \eta\mathbf{v} + \zeta\mathbf{w}$ . For these cuts,  $\xi = 0.3$ . In Cartesian coordinates,  $\mathbf{q} = (0.06, 0.21, 0.20) \text{ \AA}^{-1}$ . In reciprocal lattice units,  $\mathbf{q} = (0.94, 3.12, 1.94)$ . (c) Integrated data in the region shown in (f) taken from the in-situ 100C, 500 mA data set. (d) Fit to the data in (c). In Cartesian coordinates, the intersection is at  $\mathbf{q} = (0.07, 0.21, 0.2) \text{ \AA}^{-1}$  and in reciprocal lattice units,  $\mathbf{q} = (0.98, 3.09, 1.94)$ .

|             | h               | k               | l               |
|-------------|-----------------|-----------------|-----------------|
| S1          | $1.00 \pm 0.02$ | $3.08 \pm 0.02$ | $1.93 \pm 0.01$ |
| 100°C 000mA | $1.01 \pm 0.02$ | $3.00 \pm 0.02$ | $2.00 \pm 0.02$ |
| 100°C 300mA | $0.97 \pm 0.04$ | $3.01 \pm 0.04$ | $2.02 \pm 0.03$ |
| 100°C 500mA | $1.01 \pm 0.05$ | $3.06 \pm 0.05$ | $1.93 \pm 0.03$ |
| 400°C 000mA | $1.02 \pm 0.05$ | $2.94 \pm 0.05$ | $2.03 \pm 0.02$ |
| 400°C 950mA | $1.01 \pm 0.04$ | $3.00 \pm 0.05$ | $1.99 \pm 0.02$ |
|             | $1.00 \pm 0.04$ | $3.02 \pm 0.04$ | $1.98 \pm 0.02$ |
| S2          | $0.99 \pm 0.02$ | $3.02 \pm 0.04$ | $1.99 \pm 0.05$ |

Tab. 1: Directions (in r.l.u.) of the (132) needles in the diffuse scattering. The needle direction for each data set is determined by fitting the intersection of the needle as discussed in the text. The reported values are averaged over all needles in each summed data set. The error bars are standard deviations.

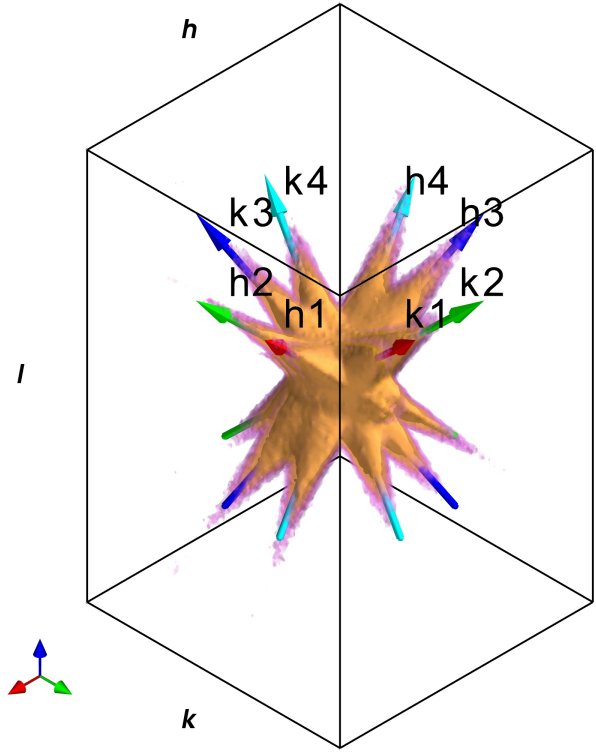

Fig. 3: Label of the different needles discussed in the text. The volumetric data are from the summed S1 dataset.

The directions of the  $k_1$  needle for all data sets are given in table 1. We call the needles  $k_1, k_2, \dots, h_1, h_2, \dots$  etc. The letter denotes which face of the Brillouin zone they intersect. The subscripts label the different needles as shown in fig. 3.  $k_1$  has all components positive. The other needles can be obtained by applying tetragonal symmetry operations.

For the (225) needles, quantitative analysis was more difficult since the intensity of the needles is weaker and decays more quickly away from the Bragg peak than the (132) needles. The (225) needles are only present in the S2 dataset, but were determined to point along (225) by fitting with same procedure described above.

## 2 Summed datasets

As discussed in the main text, qualitative analysis of the diffuse scattering data is frustrated by the structure factor: diffuse scattering around the Bragg peaks is asymmetric and varies from Brillouin zone to Brillouin zone. To aid in the analysis and visualization of the diffuse scattering, we picked all Brillouin zones showing significant diffuse scattering and summed them to a single Brillouin zone. Specifically, let  $\mathbf{Q} = \mathbf{G} + \mathbf{q}$ , with  $\mathbf{G}$  a reciprocal lattice vector labeling an extended Brillouin zone and  $\mathbf{q}$  a reduced wave vector. We selected all  $\mathbf{G}$  with significant diffuse scattering and translated them to a single Brillouin zone, then summed the data at equivalent  $\mathbf{q}$  in the chosen zones. The summed intensity for all datasets measured are presented in fig. S4.

In fig. S4, the blue vectors show the direction of current; the red vectors label the



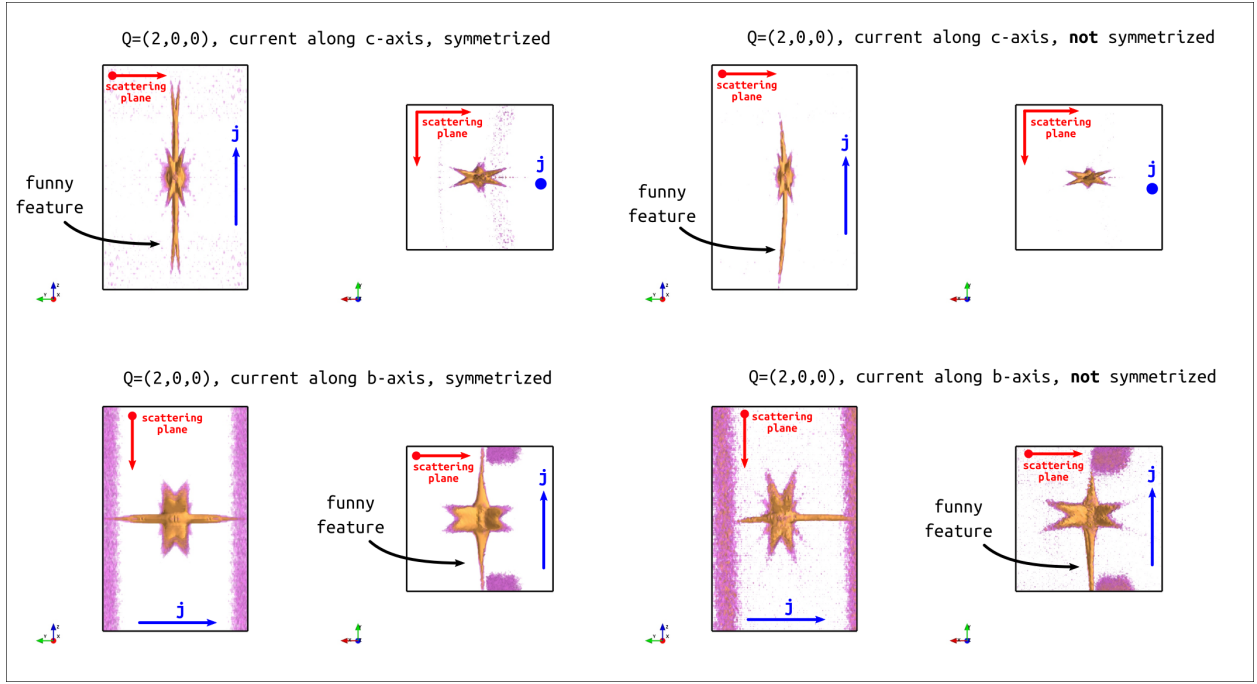

Fig. 5: Volumetric plots of diffuse scattering in the  $\mathbf{Q} = (2, 0, 0)$  and  $\mathbf{Q} = (2, 1, 0)$  zones in the raw (i.e. not summed) S1 (current along  $b$ -axis) and S2 (current along  $c$ -axis) datasets. The funny features labeled in the figures originating from saturated detectors during the experiment.

scattering plane. In the in-situ data, the current was always in the scattering plane. In the ex-situ data, the sample was mounted different for different experiments.

The fuzzy background in the in-situ datasets is scattering the furnace. The prominent diffuse scattering features are correlated with the size of the current; with increasing current, the sea-urchin like features enhance (see main text).

The funny looking features, labeled as artifacts, are a nuance of the experiments. Bragg scattering is incredibly strong and saturated the entire detector tubes, resulting in curved rods perpendicular to the scattering planes. Examples of the artifacts in the raw (i.e. not summed) S1 and S2 datasets are shown at  $\mathbf{Q} = (2, 0, 0)$  and  $\mathbf{Q} = (2, 1, 0)$  in fig. S5.

### 3 Curie-Weiss fits to magnetic susceptibility

In table 2, we provide the results of Curie-Weiss fits to the magnetic susceptibilities over the full and low temperature ranges as discussed in the main text.

### 4 Integrating data along arbitrary projections

The diffuse scattering data lie on a 3-dimensional rectilinear grid. Each element is called a *voxel*. To make 1-dimensional cuts along and perpendicular to the needles, we want to rehistogram the data. However, the needles do not point along a grid edge. MANTID [1] was

|                                   | $\chi_{ab}^p$ | $\chi_c^p$ | $\chi_{ab}^f$ | $\chi_c^f$ |
|-----------------------------------|---------------|------------|---------------|------------|
| $\mu_{eff}$ ( $\mu_B/\text{Ti}$ ) | 0.024         | 0.025      | 0.069         | 0.065      |
| (all T)                           | 0.035         | 0.061      | 0.092         | 0.087      |
| $\theta_{cw}$ (K)                 | -2.2          | -3.2       | -0.9          | -0.7       |
| (all T)                           | -7.1          | -25.6      | -3.8          | -3.6       |
| $\chi_0 \times 10^5$ (emu/mol/Oe) | 8.0           | 3.3        | 20.0          | 29.0       |
| (all T)                           | 7.8           | 2.7        | 19.0          | 28.0       |

Tab. 2: Results of fitting magnetic susceptibilities of pristine rutile  $\text{TiO}_2$  along the  $ab$  plane,  $\chi_{ab}^p$ , and along the  $c$  axis,  $\chi_c^p$  and the flashed S2 sample along the  $ab$  plane,  $\chi_{ab}^f$ , and along the  $c$  axis,  $\chi_c^f$ . We provide fits to the low-T regime ( $T \leq 50$  K) and all temperature (“all-T”).

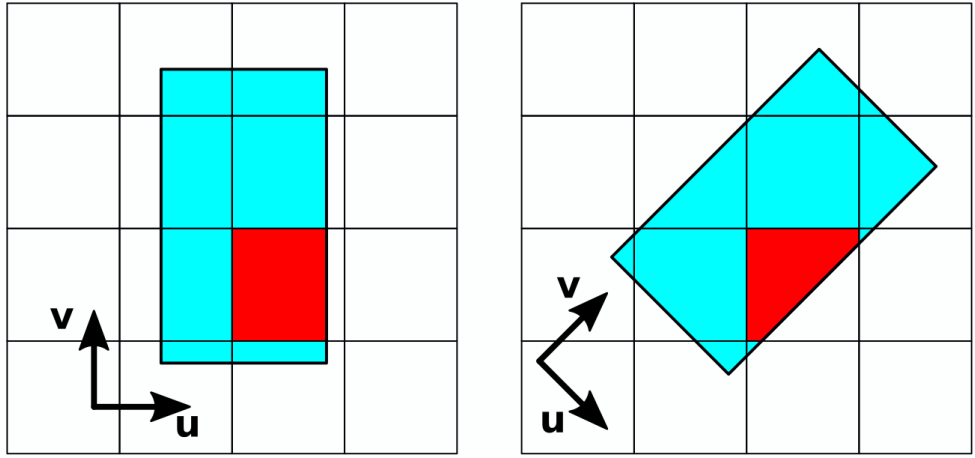

Fig. 6: Overlapping integration bins voxels. The red regions correspond to the integration weights, i.e. the “volume” of the overlap.

used for data reduction and manipulation, but as of this writing, there are no algorithms in MANTID for rehistogramming data in a direction that isn’t commensurate with the voxels.

To rehistogram the data, we define a direction in which want to integrate and specify the bin spacing in each direction. We call the directions  $\mathbf{u}$ ,  $\mathbf{v}$ , and  $\mathbf{w}$  as discussed above. The combined set  $\hat{R} = (\mathbf{u}, \mathbf{v}, \mathbf{w})$  is called a “projection” and we label the projection by  $\hat{R}$ , the matrix that transforms from the rectilinear coordinates of the voxels to the projection axes. To make 1-dimesional cuts along  $\mathbf{u}$  (“line cuts”), we rebin along  $\mathbf{u}$  and integrate over  $\mathbf{v}$  and  $\mathbf{w}$ . Each bin along  $\mathbf{u}$  is a rectangular prism and all of the voxels are rectangular prisms (see fig. S6). Each voxel that falls into a bin contributes some amount of weight. If the full voxel lies in a bin, its weight in that bin is 1. If it is partially in the bin, its weight is equal to the volume of overlap normalized by the total volume of the voxel. In the case that the binning projection is parallel to the voxel edges, calculating the weights is relatively easy. When the projection lies in an arbitrary direction, calculating the overlap between bins and voxels is mathematically straightforward but is computationally challenging. As a work around, we use an approximate strategy.

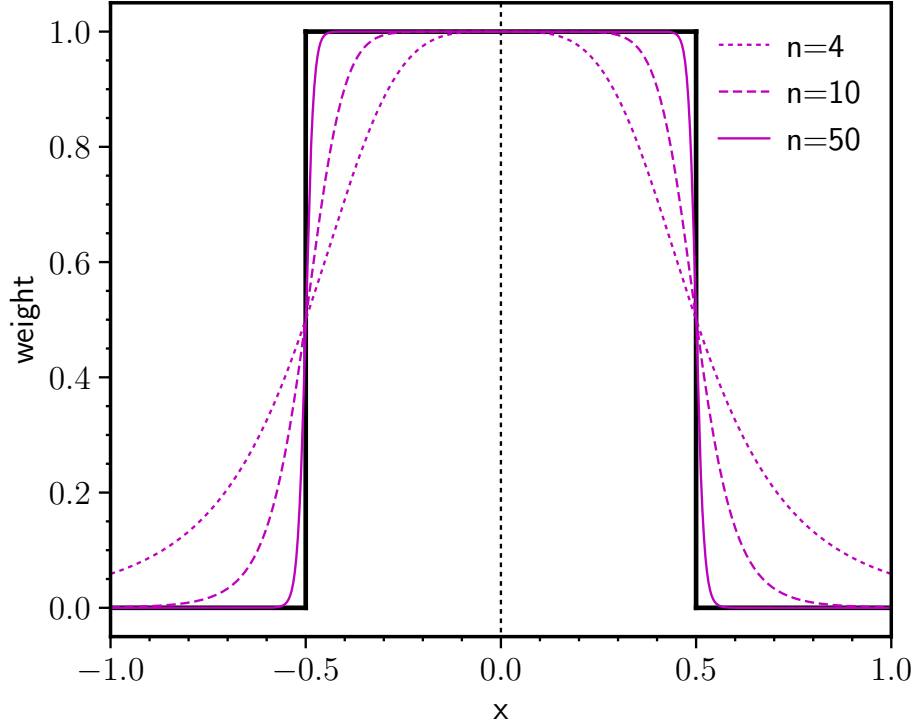

Fig. 7: 1-dimensional Butterworth function for several values of  $n$ , all with  $\Delta q = 1$  and  $q_0 = 0$ . For small  $n$ , the edge of the bin is broad. For large  $n$ , the edge is sharp.  $x_0 = 0$  and  $\Delta x = 1$ . The bold, black line is a square pulse, showing the limit  $n \rightarrow \infty$ .

Let us restate the problem in words. Consider only a single bin from here on. We want to integrate around an interesting feature in the data to improve statistics and do further analysis. Let  $\mathbf{q}_0$  be the coordinate of the feature in voxel coordinate system. We want voxels near the interesting feature (near the bin center) to contribute significantly to the integral, but voxels far away (near the bin edges) to contribute less. This is the same idea as in fig. S6. Voxels fully in the bin have weight 1, but voxels only partially in the bin have lower weight. To approximate this scheme, we define a weighting function,  $w(\mathbf{q})$ , that is 1 for voxels that are in the middle of a bin and decay to 0 near the edge of the bin.  $\mathbf{q}$  are the coordinates of the center of the voxels. A good function for this is the “Butterworth function”. Its 1-dimensional version is

$$w(q) = \left[ 1 + \left( \frac{q - q_0}{\frac{1}{2}\Delta q} \right)^n \right]^{-1}. \quad (1)$$

$q_0$  specifies the bin center and  $\Delta q$  is the bin width; it is the full-width at half-maximum (FWHM) of the Butterworth function.  $n$  is an even integer that controls how quickly the functions decays from 1 to 0 near the edge of bin. In other words, it controls how much voxels near the bin edges contribute to the integral. The 1-dimensional Butterworth function is plotted for several  $n$  in fig. S7.

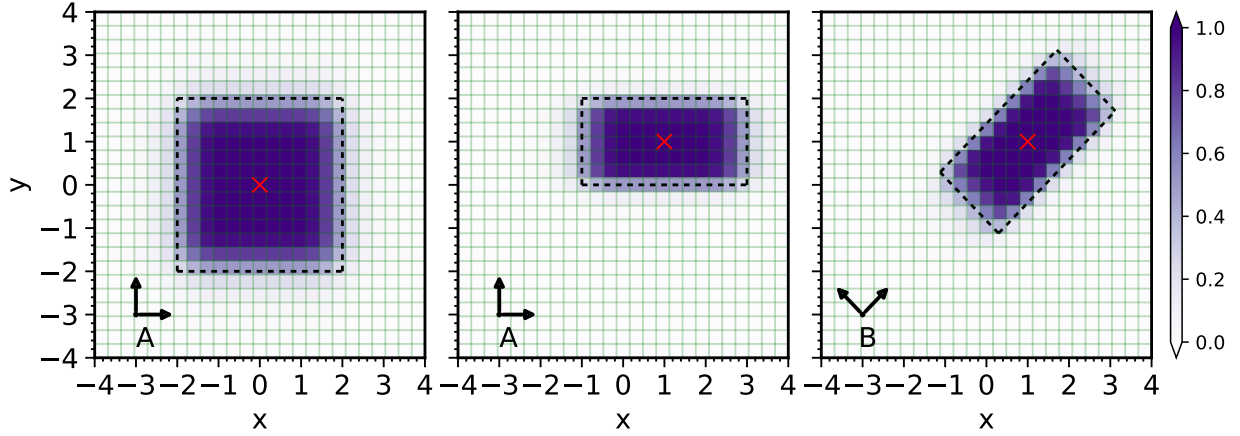

Fig. 8: 2-dimensional Butterworth function for several different widths and projections. The grid represents edges of voxels and the colormap shows the weight of each voxel in the bin; the bin edges are denoted by the dashed line. In the left panel,  $\Delta x = \Delta y = 4$  and  $x_0 = y_0 = 0$ . In the middle, the center is shifted to  $x_0 = y_0 = 1$  and the widths are  $\Delta x = 4$ ,  $\Delta y = 2$ . The projection is still parallel to the voxel edges. In the right panel, the center and widths are the same as the middle but the projection is rotated by  $45^\circ$  from the voxel axes.

The 3-dimensional generalization of the Butterworth function is

$$w(\mathbf{q}) = \left[ \left( 1 + \left( \frac{h - h_0}{\frac{1}{2}\Delta h} \right)^n \right) \left( 1 + \left( \frac{k - k_0}{\frac{1}{2}\Delta k} \right)^n \right) \left( 1 + \left( \frac{l - l_0}{\frac{1}{2}\Delta l} \right)^n \right) \right]^{-1}. \quad (2)$$

$h_0$ ,  $k_0$ , and  $l_0$  are the  $h$ ,  $k$ , and  $l$  coordinates of the bin center in Cartesian coordinates.  $\Delta h$ ,  $\Delta k$ , and  $\Delta l$  are the widths of the bins along the directions parallel to  $h$ ,  $k$ , and  $l$ .

To use the Butterworth function to rehistrogram, we define the coordinate of the bin center,  $\mathbf{q}_0 = (h_0, k_0, l_0)^T$ , the widths  $\Delta \mathbf{q} = (\Delta h, \Delta k, \Delta l)^T$ , and projection directions  $\mathbf{u}$ ,  $\mathbf{v}$ ,  $\mathbf{w}$  based on the feature we are interested in. The widths are parallel to the projection axes. To integrate along a particular direction, we rotate the voxel coordinate system to be aligned with the projection directions. We assume the voxel coordinates are orthonormal so that the rotation matrix  $\hat{R} = (\mathbf{u}, \mathbf{v}, \mathbf{w})$  is just the matrix of projection vectors. Since the rotation is around the origin, to integrate along a feature that is offset from the origin at position  $\mathbf{q}_0$ , we must first translate the center of the feature to the origin. Then  $\mathbf{q}' = \hat{R}(\mathbf{q} - \mathbf{q}_0)$ . We evaluate the Butterworth function for the new coordinates  $\mathbf{q}'$ , giving us the weights of the coordinates originally at  $\mathbf{q}$  that fall in our bin centered on  $\mathbf{q}_0$ .

We provide a 2-dimensional example of this approximate procedure to calculate weights in fig. S8. The 2-dimensional version of the Butterworth is an obvious generalization of eq. S2. The weights are denoted by the colormap. Even in the case where the projection axes are rotated, the voxels at the edge of the bin indeed contribute less to the integration ( $w < 1$ ) while voxels in the middle of the bin contribute most strongly ( $w = 1$ ). This is the desired outcome.

The data in fig. S2 are integrated using this scheme; the weights calculated by the

| $\text{\AA}^{-1}$ | $k_1$  | $k_2$  | $k_3$  | $k_4$  | $h_1$  | $h_2$  | $h_3$  | $h_4$  |
|-------------------|--------|--------|--------|--------|--------|--------|--------|--------|
| $\sigma$          | 0.0762 | 0.0762 | 0.0778 | 0.0769 | 0.0569 | 0.0582 | 0.0545 | 0.0543 |

Tab. 3: Experimental resolution in the direction of each needle determined by fitting line cuts through diffuse scattering from a pristine  $\text{TiO}_2$  crystal. The results,  $\sigma$ , are FWHM of Gaussians, in  $\text{\AA}^{-1}$ , fit to the data.

Butterworth function are shown in fig. S2 e) and f). As another example, we plot the integration weights for the line cuts along the  $h_3$  needle at the  $\mathbf{Q} = (2, 1, 2)$  in fig. S9 and for the line cuts perpendicular to the  $\mathbf{Q} = (2, 1, 2)$   $h_3$  needle in figs. S10 and S11.

We used method described here, with  $n = 40$ , for all line cuts in this supplementary document and in the main text.

## 5 Resolution

The experimental resolution is estimated by fitting the diffraction data from a pristine crystal under the same experimental conditions as the S1 data sets (i.e. room temperature with out a furnace and the same crystal orientation). Pristine data are plotted alongside S1 data in figs. S12, S13, S14, S15, S16, and S17. We attempted to fit the pristine data with Voigt functions; however, the result was vanishing Lorentzian component. The Bragg peaks in the pristine data are best described by pure Gaussians. The resolution is anisotropic, so it is useful to estimate it along the direction of each needle. We fit line cuts in the direction of each needled through multiple pristine Bragg peaks and averaged over the Bragg peaks. The results characterizing the resolution are presented in table 3.

## 6 Line cuts through the diffuse scattering

To show the asymmetry of the diffuse scattering around Bragg peaks and to show structure factor of the diffuse scattering, we pick a handful of symmetry-inequivalent Bragg points and plot line cuts along each needle in the S1 data set. Figs. S12, S13, S14, S15, S16, and S17 show the data at the select points. Interestingly, even though the electric field in the  $ab$  plane breaks the tetragonal symmetry, the data still exhibit tetragonal symmetry within numerical error. To improve statistics, all line cuts that are equivalent under  $Pmmm$  symmetry are averaged.

Needles in reciprocal space correspond to pancake-like correlations in real space. Fitting the needles tells us the size of the correlated regions in real space: specifically, the decay length of the diffuse scattering is reciprocal to the size of the correlations in real space. For pancake-like correlations, the decay length along the needle describes the correlation length between defect planes and the decay length perpendicular to the needles describes the size of the correlations in the planes.

Along the needles, diffuse scattering tails were fit with a Voigt function with Lorentzian full-width at half-maximum (FWHM)  $\Gamma_{\parallel}$  and Gaussian standard deviation  $\sigma_{\parallel}$ . The Lorentzian component corresponds to the correlations, with the Gaussian part corresponding to resolution broadening. Near each Bragg peak, multiple needles intersect and the fit along a

particular needle in this region isn't meaningful. We accounted for the intersection of multiple needles at the Bragg peak by adding an additional Gaussian with standard deviation  $\sigma_B$ . The width and amplitude of the Gaussian at the Bragg peak was the same for all needles at a given peak: i.e. all needles intersecting a given Bragg peak were fit simultaneously. The background was approximated by constant offset,  $s$ . All reciprocal lengths have units  $\text{\AA}^{-1}$ . Because the structure factor is asymmetric, each side of the peak was fit separately.

The results of fitting the line cuts through the S1 data along the needles are shown in figs. S20, S21, S22, S23, S24, and S25. Averaging over all Lorentzian fits, we estimate the correlation length perpendicular to the defects to be  $46.62 \text{ \AA}$ .

We also made line cuts perpendicular to the needles to show the width. These are shown in figs. S19 and S18 for select Bragg peaks. To estimate the size of the pancake-like defects, we fit the widths of the needles. Since multiple needles intersect near the Bragg peaks, the fits near the Bragg peaks aren't meaningful. We focused on the needles sufficiently far from the Bragg peaks to avoid spurious fits, but the signal to background ratio is poor and the fits were difficult. To make the fits as simple as possible, we assumed a pure Lorentzian. The results of fitting cuts perpendicular to the needles are shown in figs. S26, S27, and S28.

The different curves correspond to cuts at different distances from the Bragg peaks.  $\Gamma_{\perp}$  is the FWHM of the Lorentzian fit perpendicular to the needle. The fits vary from  $0.0004 \text{ \AA}^{-1}$  to  $0.0142 \text{ \AA}^{-1}$  (two orders of magnitude) depending on how close to the Bragg peaks and along which direction we look. These fits are resolution limited and large variation in the fitting frustrates the interpretation. Moreover, neglecting the Gaussian part of the Voigt forces the Lorentzian width to be overestimated. Still, if we assume a representative width of  $0.005 \text{ \AA}^{-1}$ , then the sizes of the defects in real space are approximately  $\sim 200 \text{ \AA}$ .

## 7 Momentum dependence of diffuse scattering

We show colormaps of the diffuse scattering in the S1 dataset for several  $K$  values. Fig. S29 shows diffuse scattering at integer  $K$  values, showing how the structure factor evolves in reciprocal space. Fig. S30 shows several  $K$  values around  $K = 1$  (rlu), showing how the diffuse scattering needles disperse near Bragg peaks.

## 8 Current dependence of diffuse scattering

Line cuts along the diffuse scattering needles at several select Bragg peaks for several current densities are presented in the main text. In fig. S31, we show color maps of the same datasets across a larger region of reciprocal space.

## References

- [1] O. Arnold et al. "Mantid—Data analysis and visualization package for neutron scattering and  $\mu$  SR experiments". In: *Nuclear Instruments and Methods in Physics Research Section A: Accelerators, Spectrometers, Detectors and Associated Equipment* 764 (2014),

pp. 156–166. ISSN: 0168-9002. DOI: <https://doi.org/10.1016/j.nima.2014.07.029>.  
URL: <http://www.sciencedirect.com/science/article/pii/S0168900214008729>.

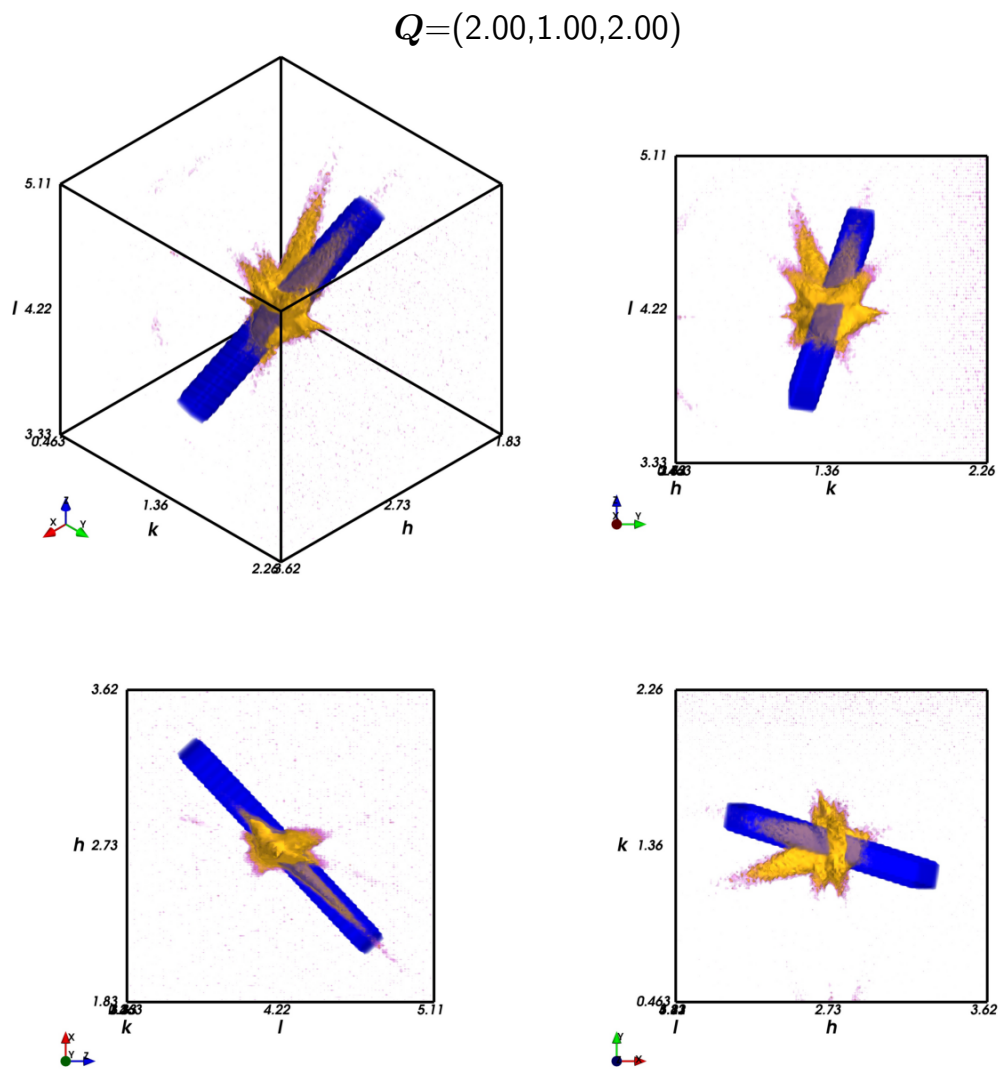

Fig. 9: Integration weights for a line cut along the  $h_3$  needle (“along  $\mathbf{u}$ ”) at the  $Q = (2, 1, 2)$  Bragg point (fig. S14). Bins along the needle are  $0.05\text{\AA}^{-1}$  thick and are integrated  $\pm 0.075\text{\AA}^{-1}$  in the perpendicular direction.

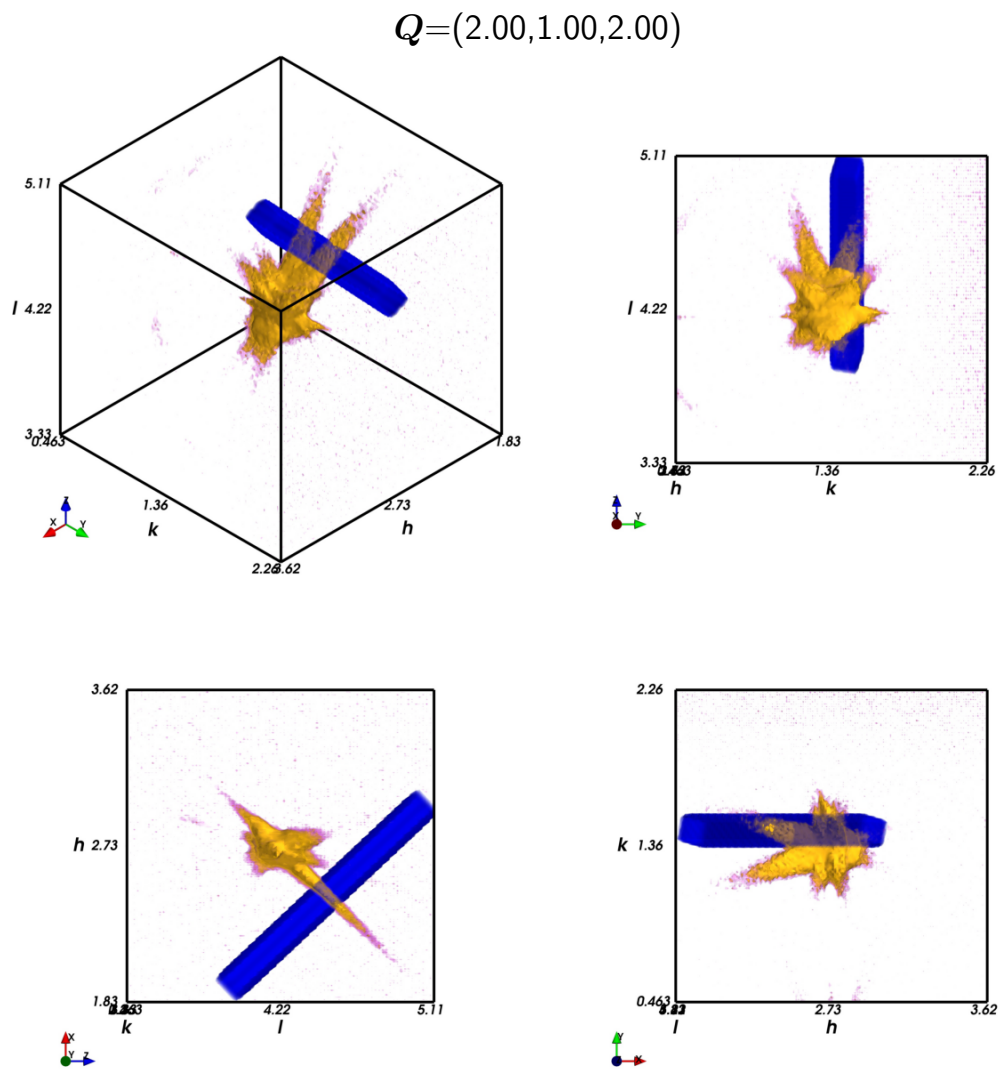

Fig. 10: Integration weights for a line cut perpendicular to the  $h_3$  needle (“along  $\mathbf{v}$ ”) at the  $Q = (2, 1, 2)$  Bragg point (fig. S14. Bins along the needle are  $0.05\text{\AA}^{-1}$  thick and are integrated  $\pm 0.075\text{\AA}^{-1}$  in the perpendicular direction. The cut is offset from the Bragg peak by a distance  $\xi = 0.3\text{\AA}^{-1}$  along  $\mathbf{u}$ .

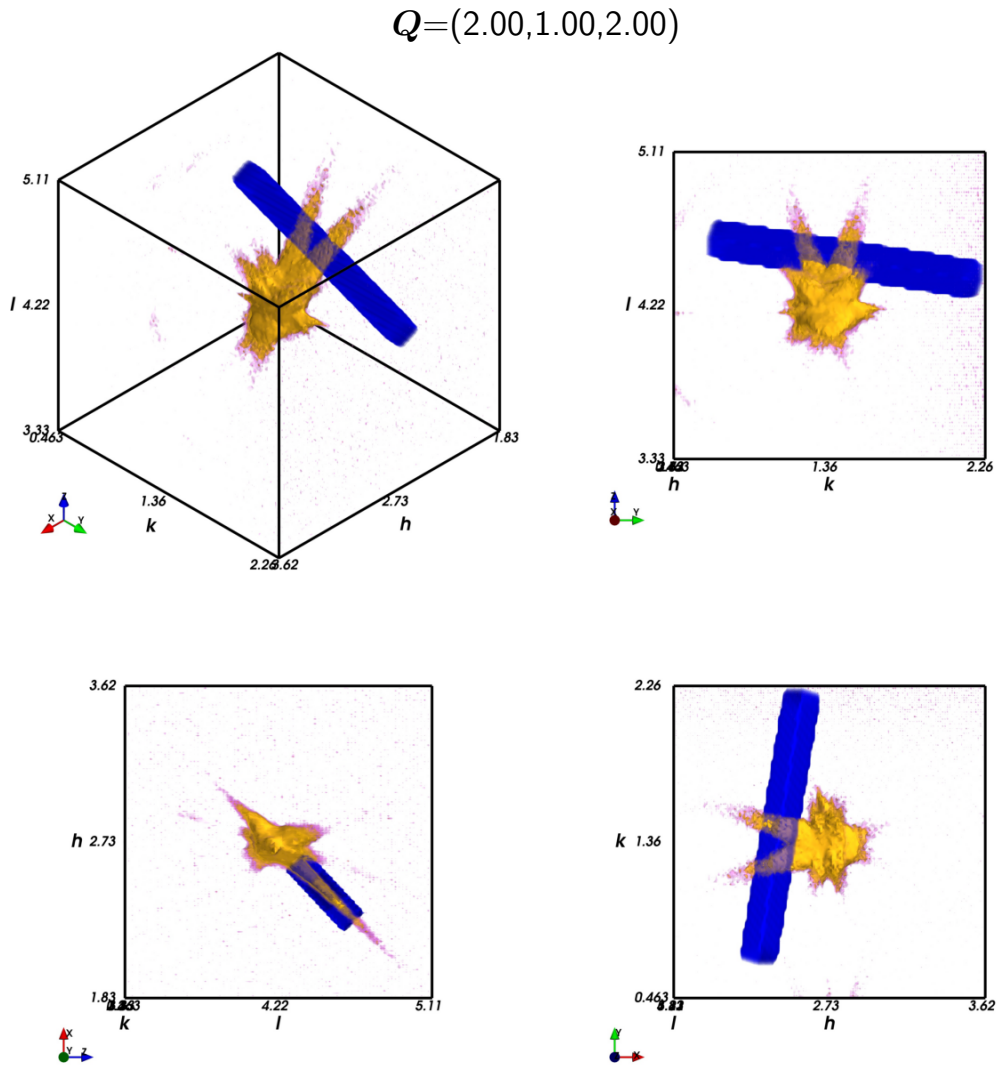

Fig. 11: Integration weights for a line cut perpendicular to the  $h_3$  needle (“along  $\mathbf{w}$ ”) at the  $Q = (2, 1, 2)$  Bragg point (fig. S14. Bins along the needle are  $0.05\text{\AA}^{-1}$  thick and are integrated  $\pm 0.075\text{\AA}^{-1}$  in the perpendicular direction. The cut is offset from the Bragg peak by a distance  $\xi = 0.3\text{\AA}^{-1}$  along  $\mathbf{u}$ .

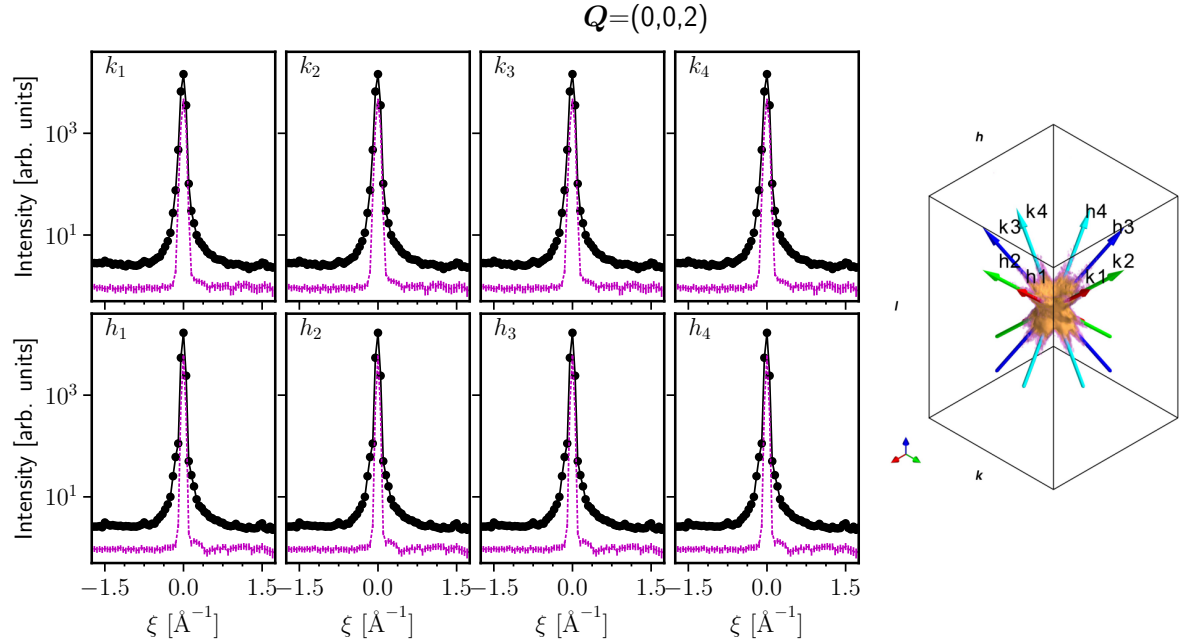

Fig. 12: Line cuts along the diffuse scattering needles at the  $Q = (0, 0, 2)$  point in the S1 data set. The data are integrated  $0.05\text{\AA}^{-1}$  along the cut and  $\pm 0.075\text{\AA}^{-1}$  perpendicular to the cut. The volumetric plot of the data in this zone labels the needles. The solid black line with circular markers is diffuse scattering from the S1 crystal; the broken magenta line is scattering from a pristine crystal.

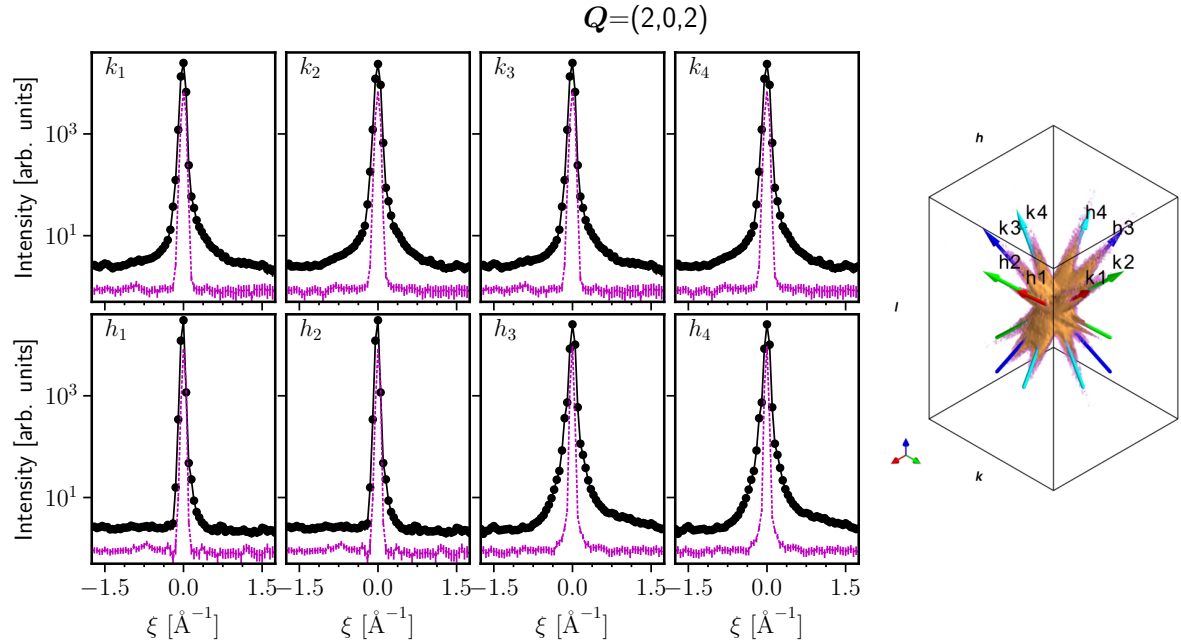

Fig. 13: Line cuts along the diffuse scattering needles at the  $Q = (2, 0, 2)$  point in the S1 data set. The binning and legend is the same as fig. S12.

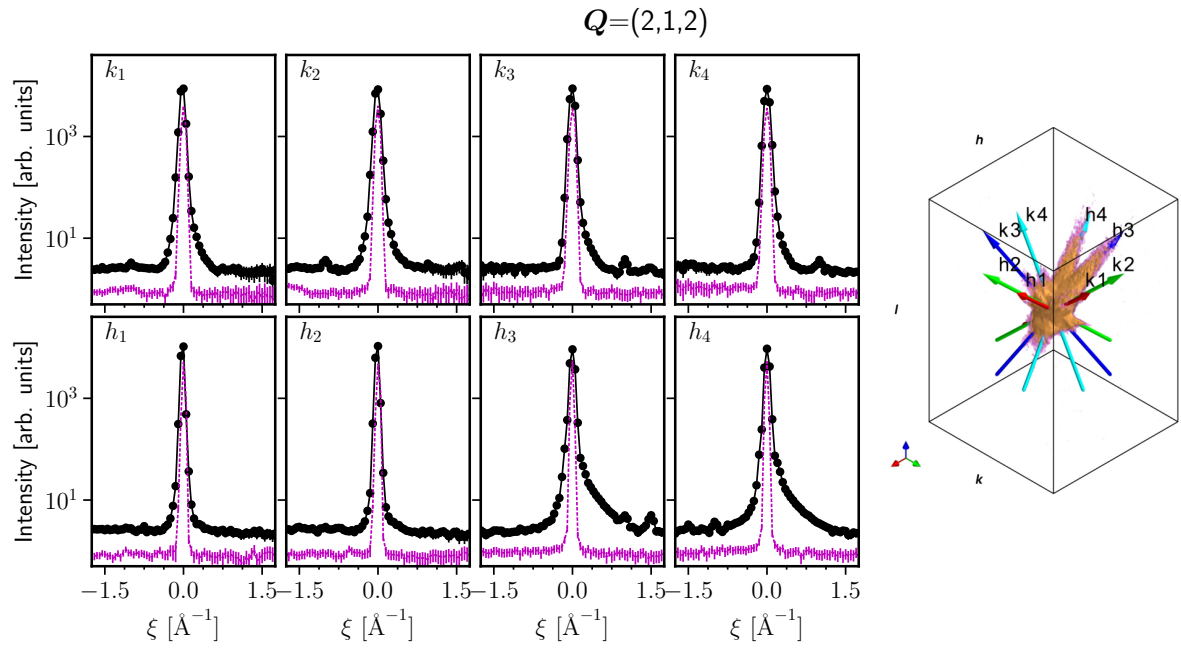

Fig. 14: Line cuts along the diffuse scattering needles at the  $Q = (2, 1, 2)$  point in the S1 data set. The binning and legend is the same as fig. S12.

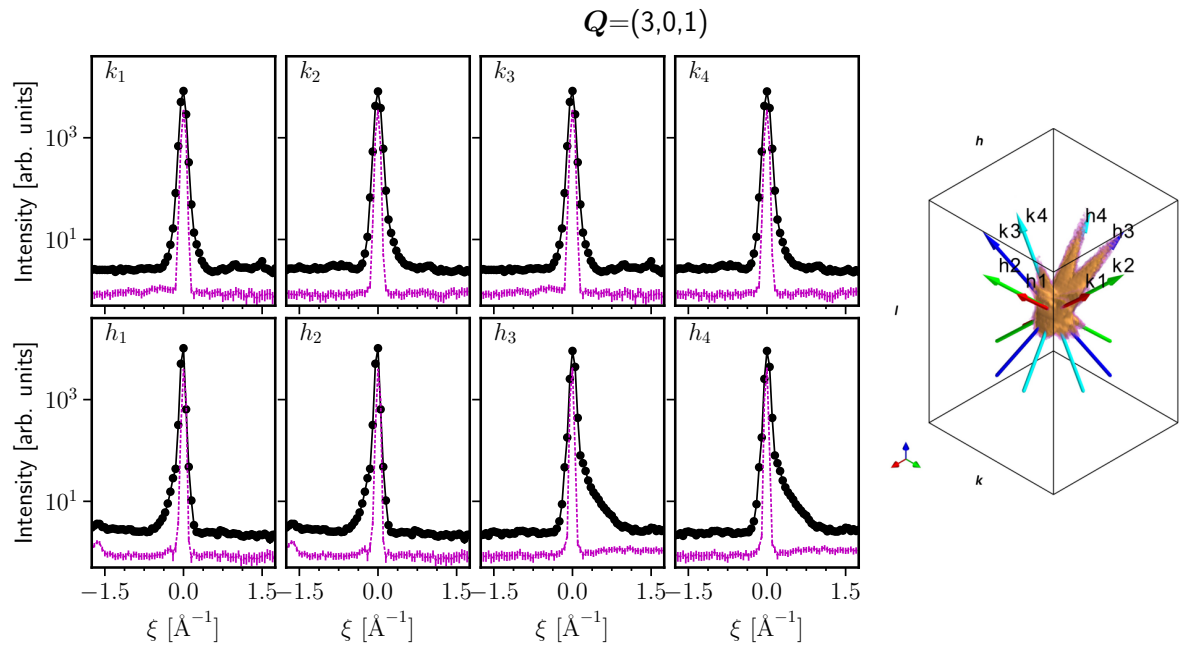

Fig. 15: Line cuts along the diffuse scattering needles at the  $Q = (3, 0, 1)$  point in the S1 data set. The binning and legend is the same as fig. S12.

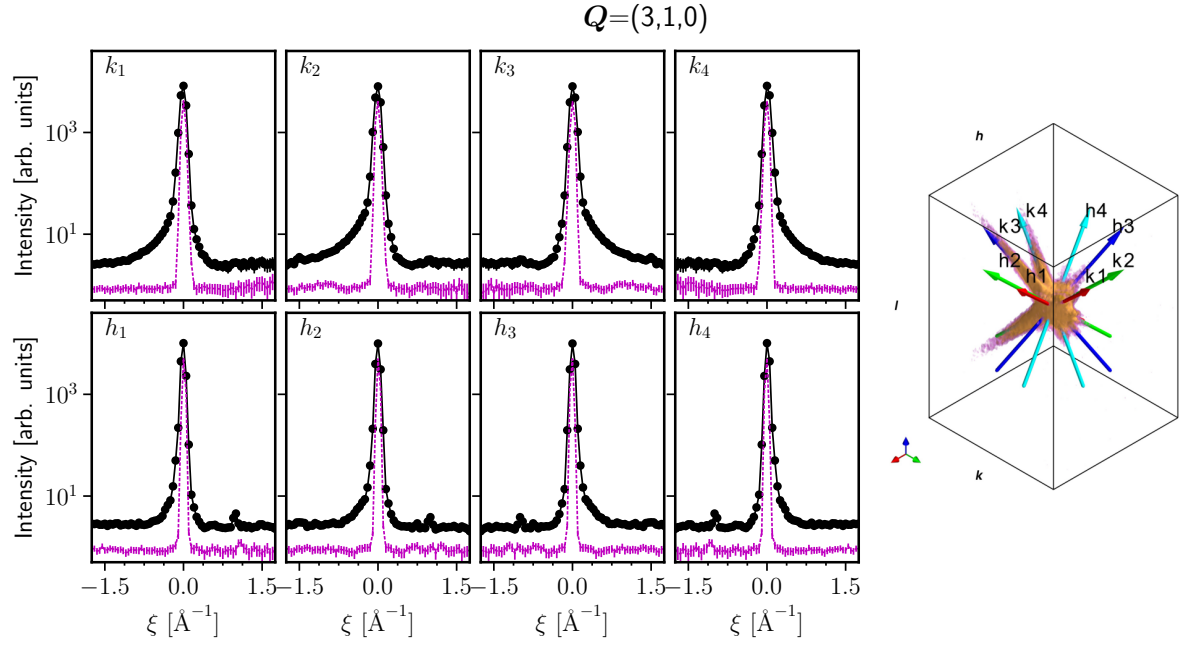

Fig. 16: Line cuts along the diffuse scattering needles at the  $Q = (3, 1, 0)$  point in the S1 data set. The binning and legend is the same as fig. S12.

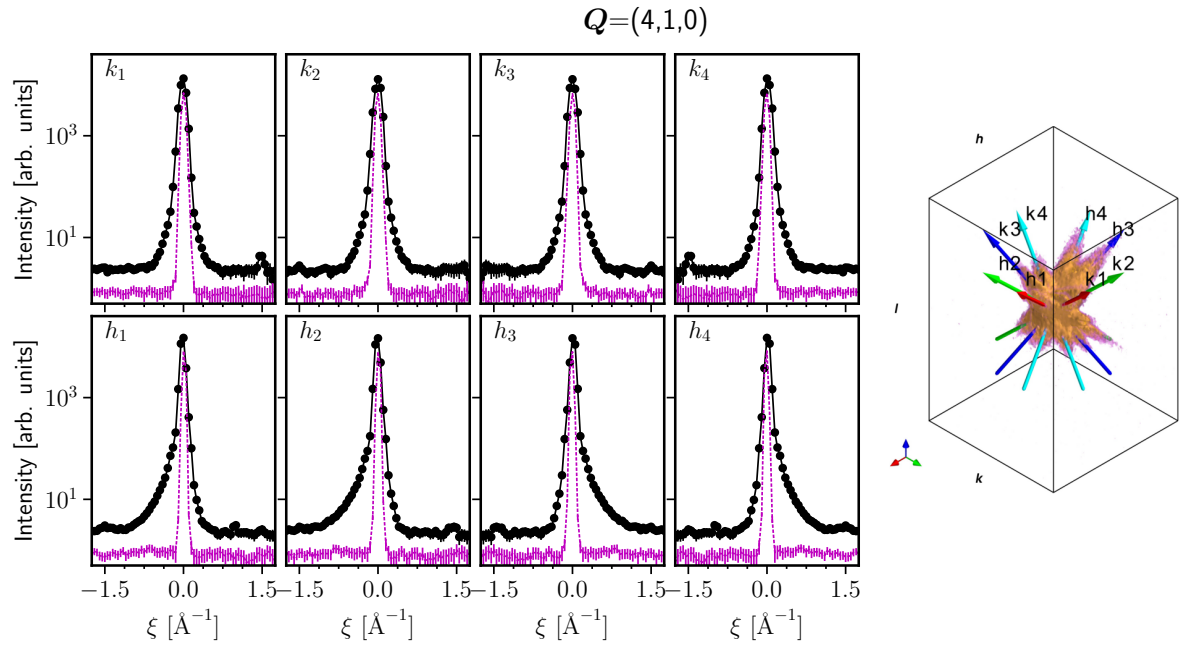

Fig. 17: Line cuts along the diffuse scattering needles at the  $Q = (4, 1, 0)$  point in the S1 data set. The binning and legend is the same as fig. S12.

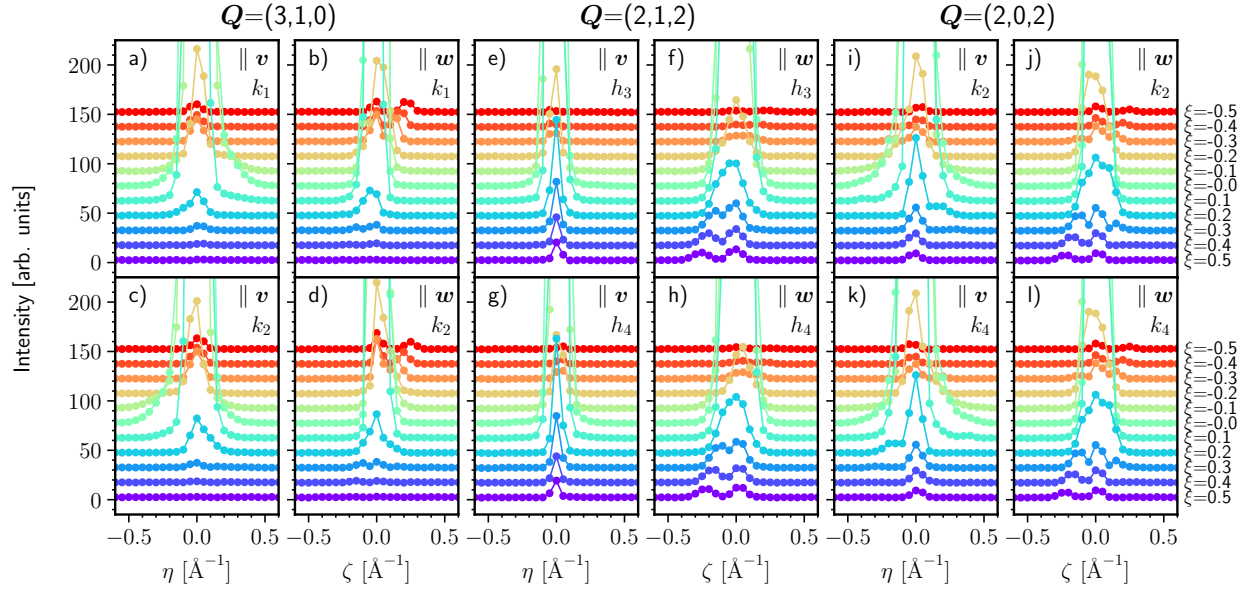

Fig. 18: Cuts perpendicular to the diffuse scattering needles near the Bragg peaks at  $\mathbf{Q} = (3, 1, 0)$  a)-d),  $\mathbf{Q} = (2, 1, 2)$  e)-h), and  $\mathbf{Q} = (2, 0, 2)$  i)-l). a), c), e), g), i), and k) are parallel to  $\mathbf{v}$  and b), d), f), h), j), and l) are parallel to  $\mathbf{w}$ ;  $\mathbf{v}$  and  $\mathbf{w}$  are mutually orthogonal vectors perpendicular to the needle. Which needle is labeled in each panel.

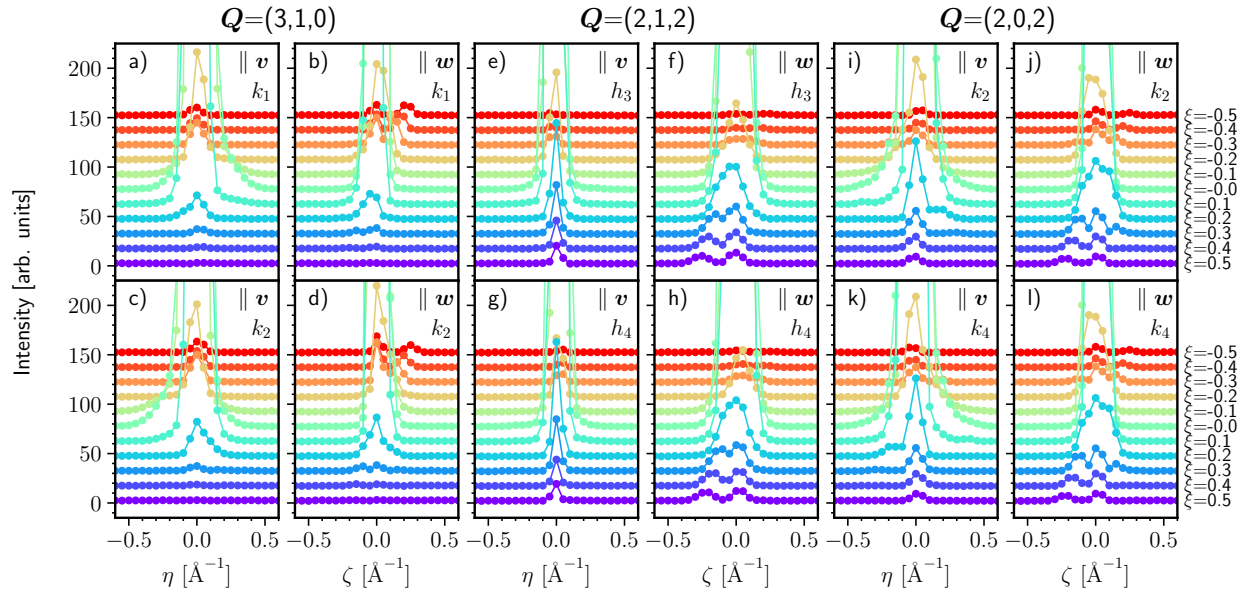

Fig. 19: Cuts perpendicular to the diffuse scattering needles near the Bragg peaks at  $\mathbf{Q} = (3, 1, 0)$  a)-d),  $\mathbf{Q} = (2, 1, 2)$  e)-h), and  $\mathbf{Q} = (2, 0, 2)$  i)-l). a), c), e), g), i), and k) are parallel to  $\mathbf{v}$  and b), d), f), h), j), and l) are parallel to  $\mathbf{w}$ ;  $\mathbf{v}$  and  $\mathbf{w}$  are mutually orthogonal vectors perpendicular to the needle. Which needle is labeled in each panel.

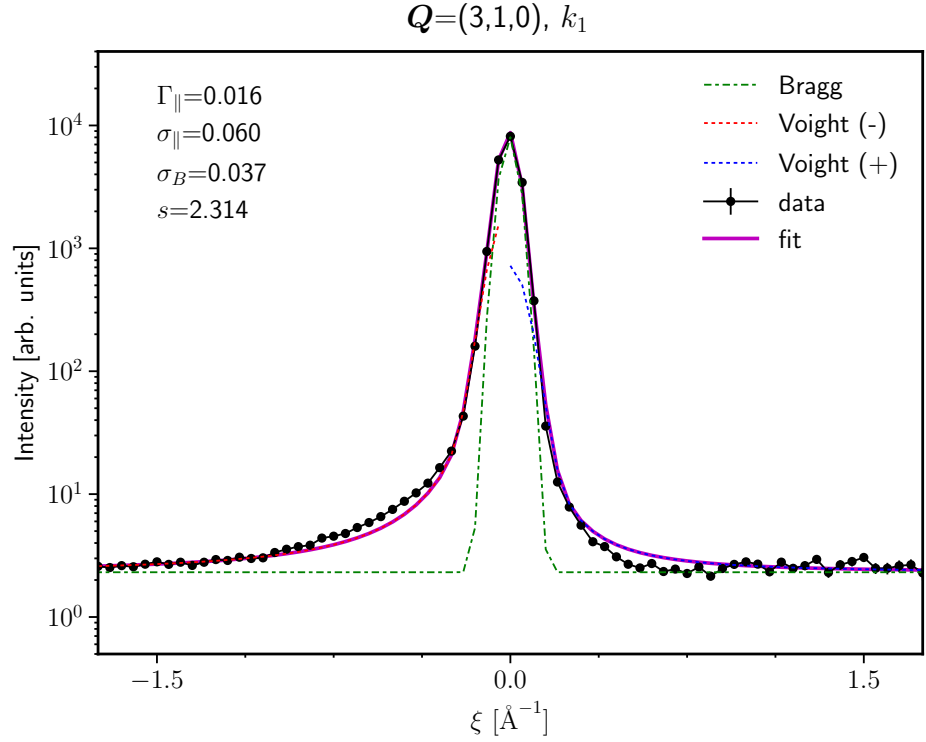

Fig. 20: Results of fitting the length of the  $k_1$  needle at the  $\mathbf{Q} = (3, 1, 0)$  Bragg peak. The tails were fit with a Voigt function with Lorentzian FWHM  $\Gamma_{||}$  and Gaussian standard deviation  $\sigma_{||}$ . The intersection of all needles at the center of the Bragg peak was approximated by Gaussian with standard deviation  $\sigma_B$ . The background was approximated by constant offset,  $s$ . Because the structure factor is asymmetric, each side of the peak was fit separately. All quantities have units  $\text{\AA}^{-1}$ .

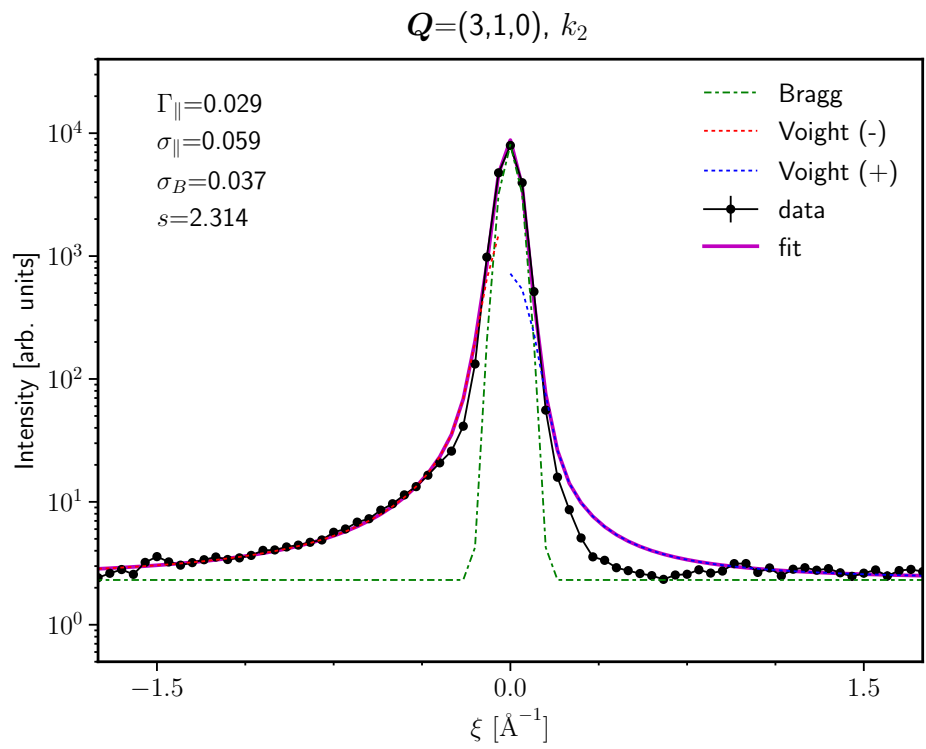

Fig. 21: Results of fitting length of the  $k_2$  needle at the  $Q = (3,1,0)$  Bragg peak. The description is the same as fig. S20.

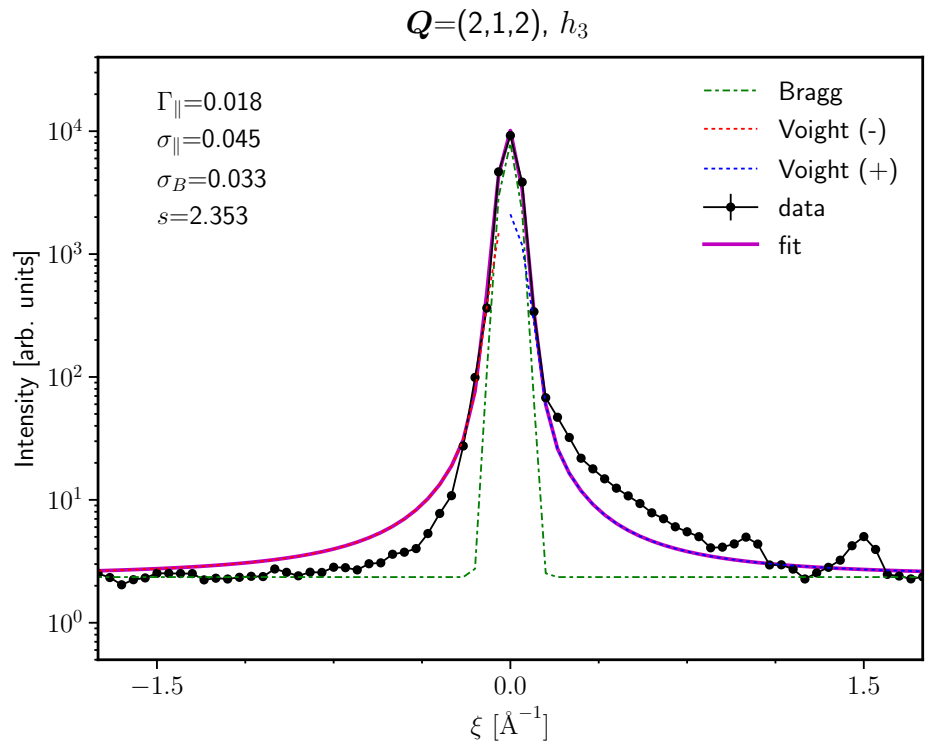

Fig. 22: Results of fitting length of the  $h_3$  needle at the  $Q = (2,1,2)$  Bragg peak. The description is the same as fig. S20.

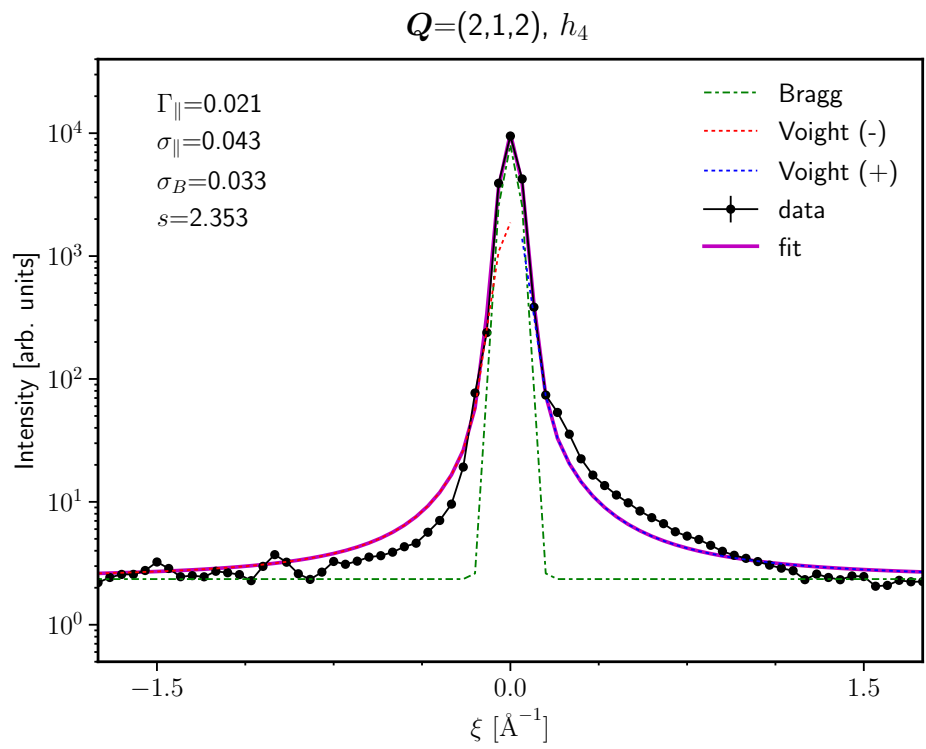

Fig. 23: Results of fitting length of the  $h_4$  needle at the  $Q = (2,1,2)$  Bragg peak. The description is the same as fig. S20.

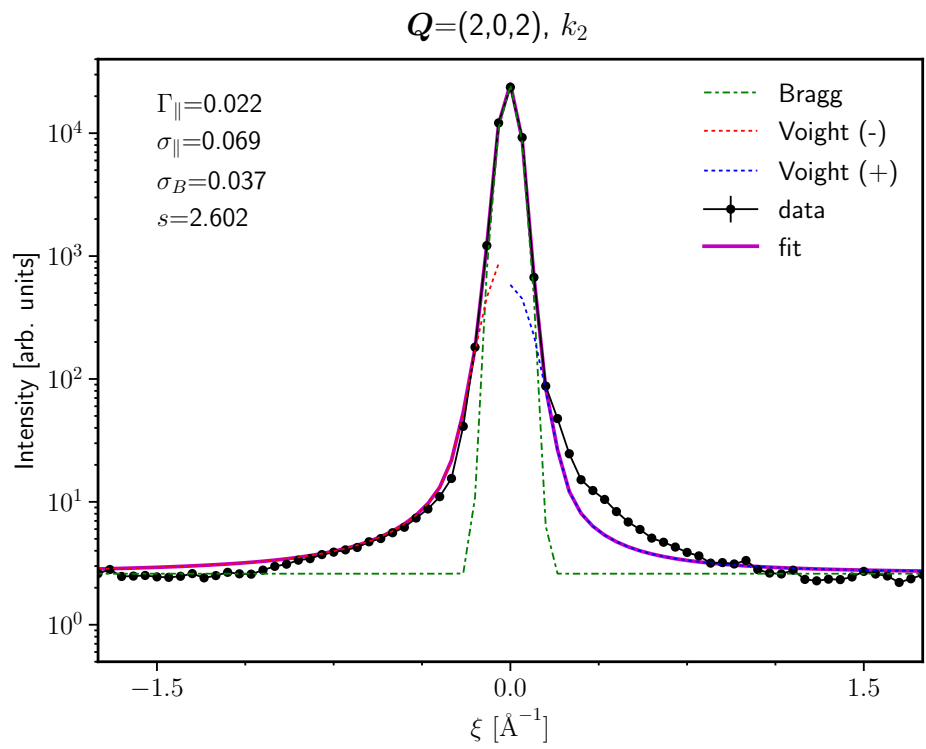

Fig. 24: Results of fitting length of the  $k_2$  needle at the  $\mathbf{Q} = (2,0,2)$  Bragg peak. The description is the same as fig. S20.

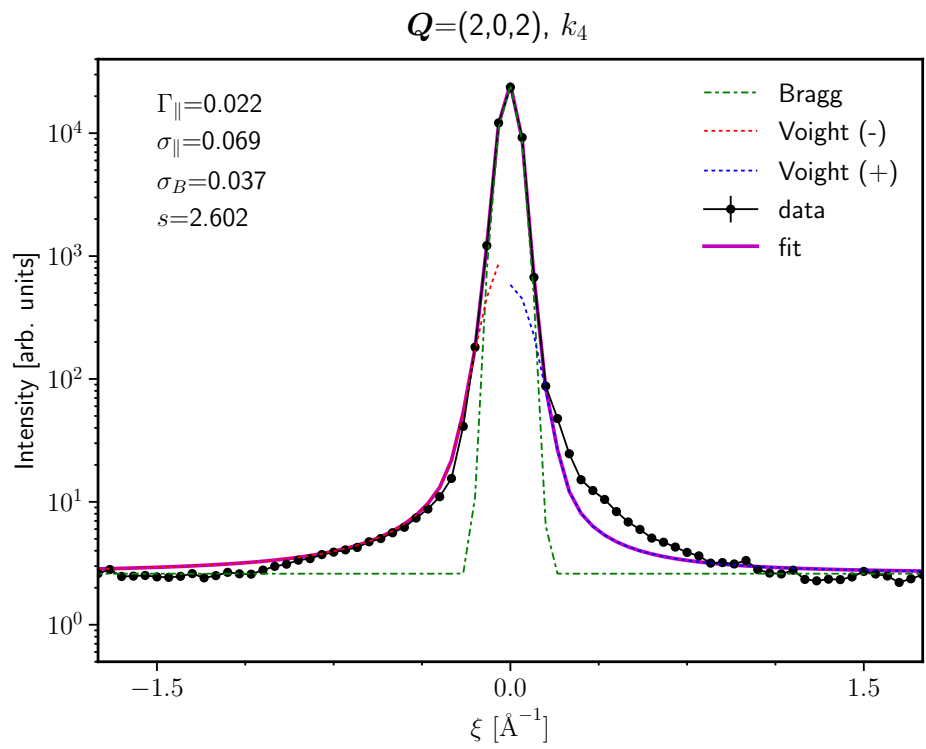

Fig. 25: Results of fitting length of the  $k_4$  needle at the  $Q = (2,0,2)$  Bragg peak. The description is the same as fig. S20.

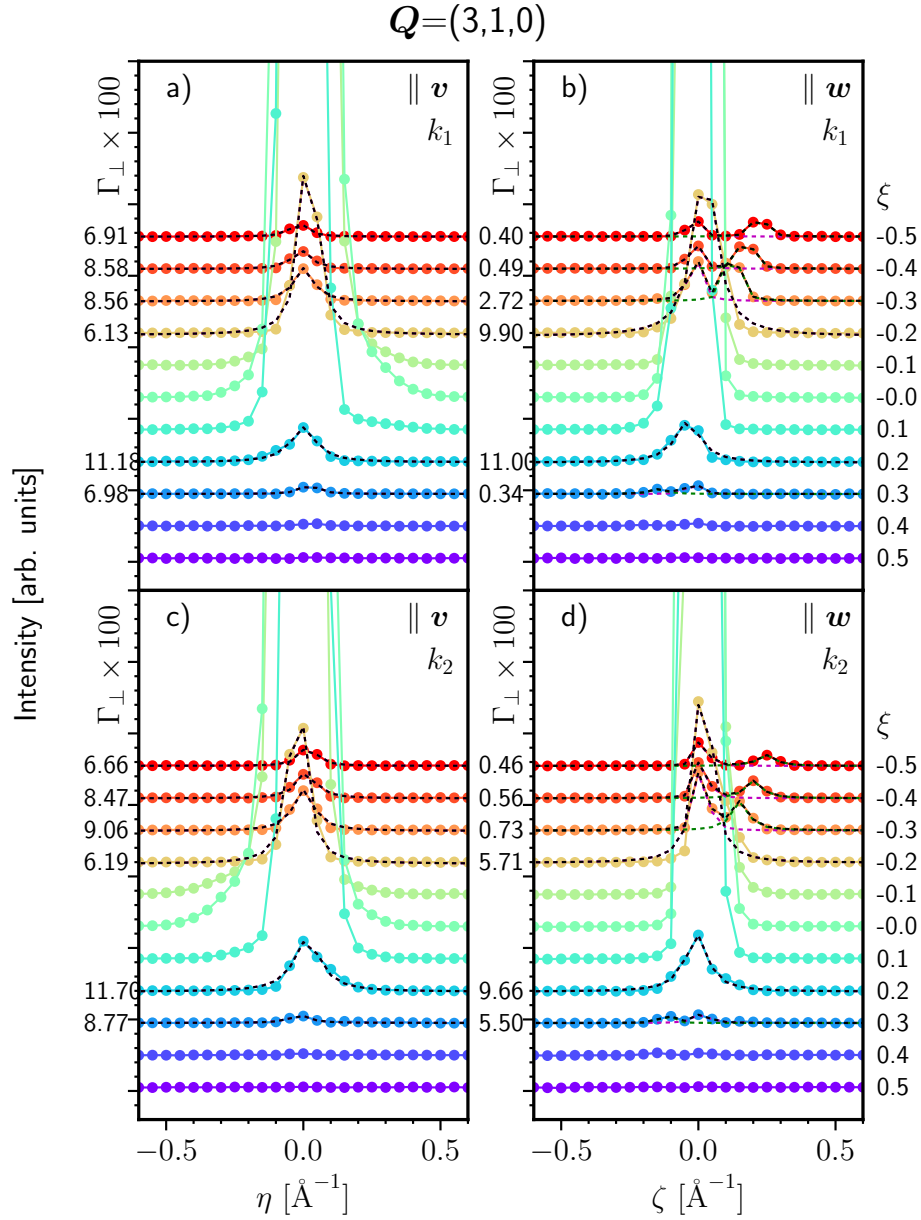

Fig. 26: Result of fitting the width of the  $k_1$  (a,b) and  $k_2$  (c,d) needles at the  $Q = (3, 1, 0)$  Bragg peak.  $\Gamma_{\perp}$  is the Lorentzian FWHM of the width of the needle in  $\text{\AA}^{-1}$ . a) and c) are along  $\mathbf{v}$  and b) and d) are along  $\mathbf{w}$ .  $\xi$  is distance ( $\text{\AA}^{-1}$ ) along  $\mathbf{u}$  from the Bragg peak (see figs. S10 and S11).

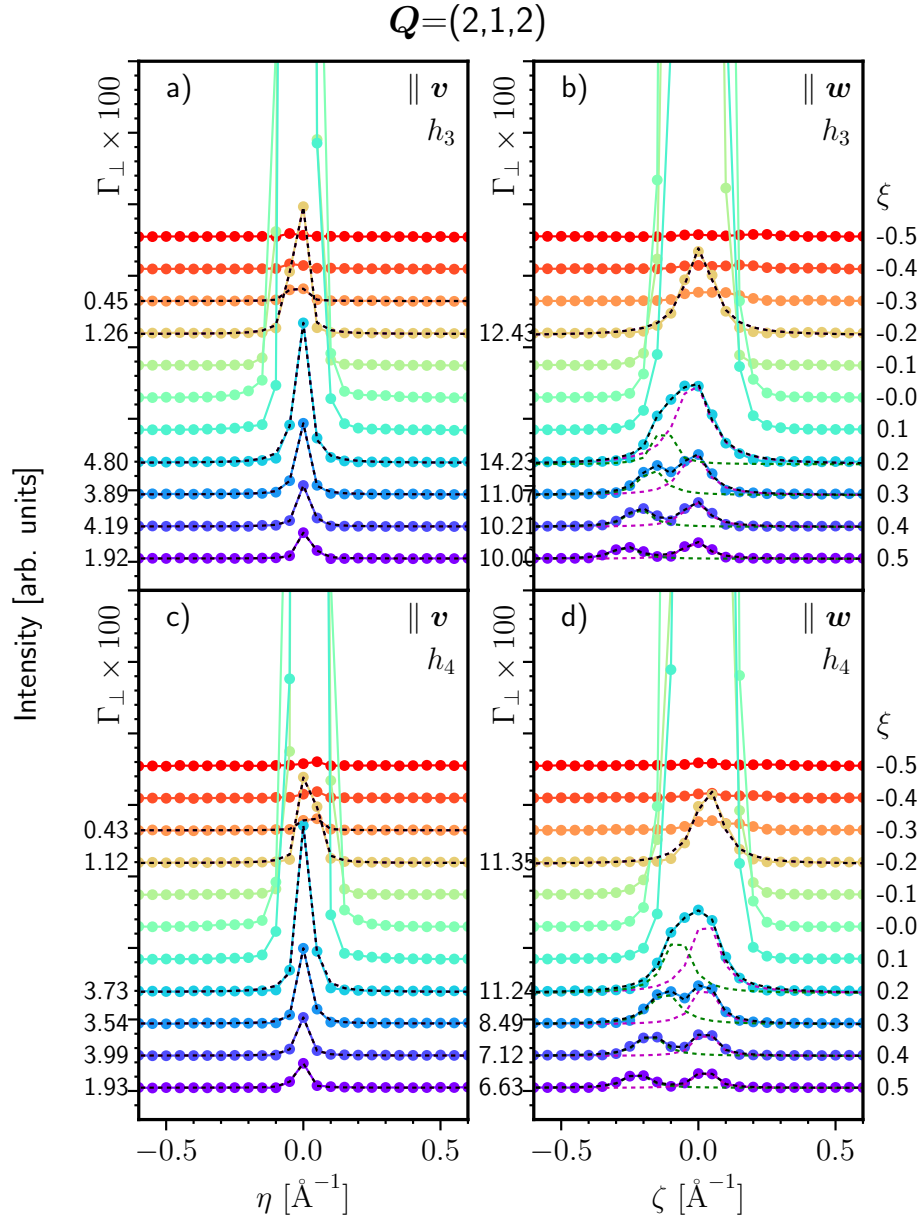

Fig. 27: Result of fitting the width of the  $h_3$  (a,b) and  $h_4$  (c,d) needles at the  $Q = (2, 1, 2)$  Bragg peak.  $\Gamma_{\perp}$  is the Lorentzian FWHM of the width of the needle in  $\text{\AA}^{-1}$ . a) and c) are along  $\mathbf{v}$  and b) and d) are along  $\mathbf{w}$ .  $\xi$  is distance ( $\text{\AA}^{-1}$ ) along  $\mathbf{u}$  from the Bragg peak (see figs. S10 and S11).

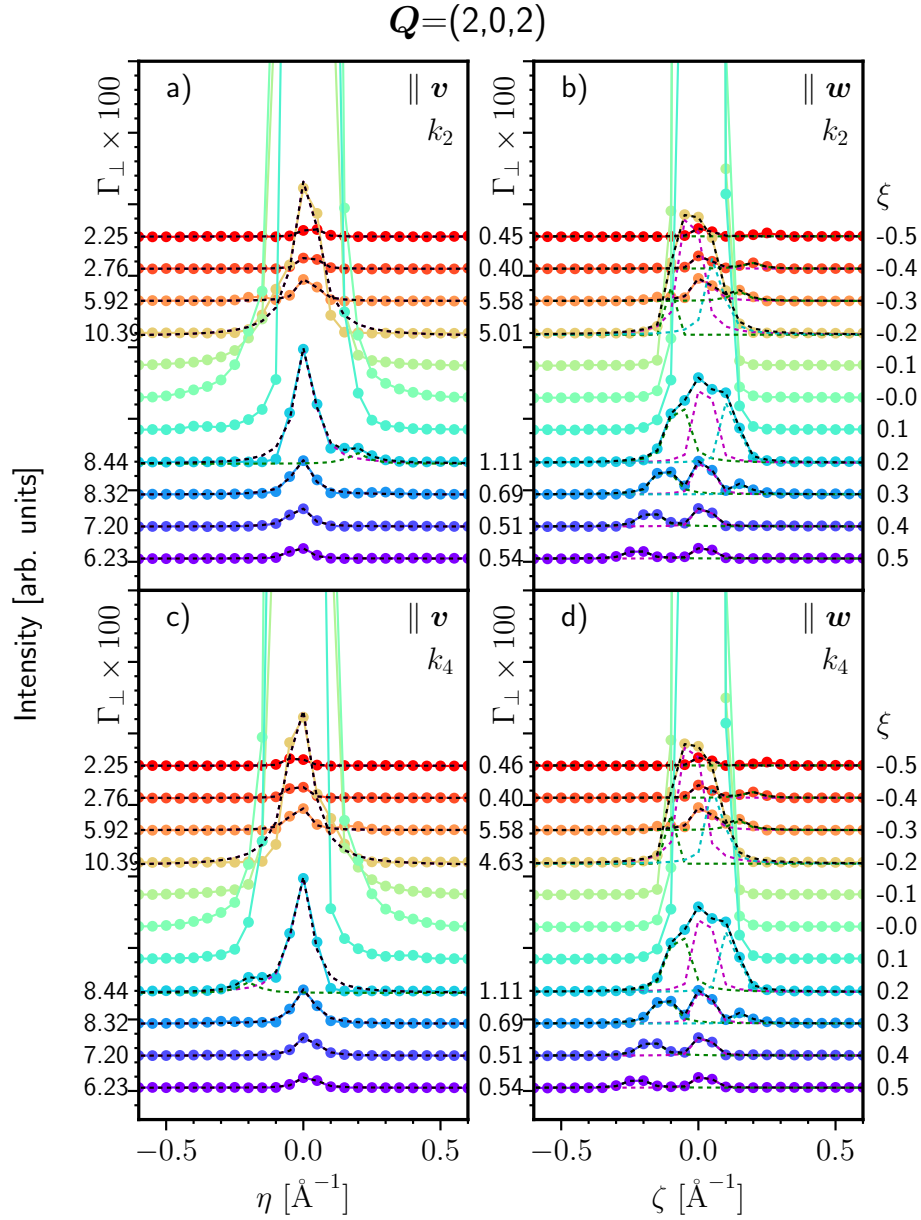

Fig. 28: Result of fitting the width of the  $k_2$  (a,b) and  $k_4$  (c,d) needles at the  $Q = (2, 0, 2)$  Bragg peak.  $\Gamma_{\perp}$  is the Lorentzian FWHM of the width of the needle in  $\text{\AA}^{-1}$ . a) and c) are along  $\mathbf{v}$  and b) and d) are along  $\mathbf{w}$ .  $\xi$  is distance ( $\text{\AA}^{-1}$ ) along  $\mathbf{u}$  from the Bragg peak (see figs. S10 and S11).

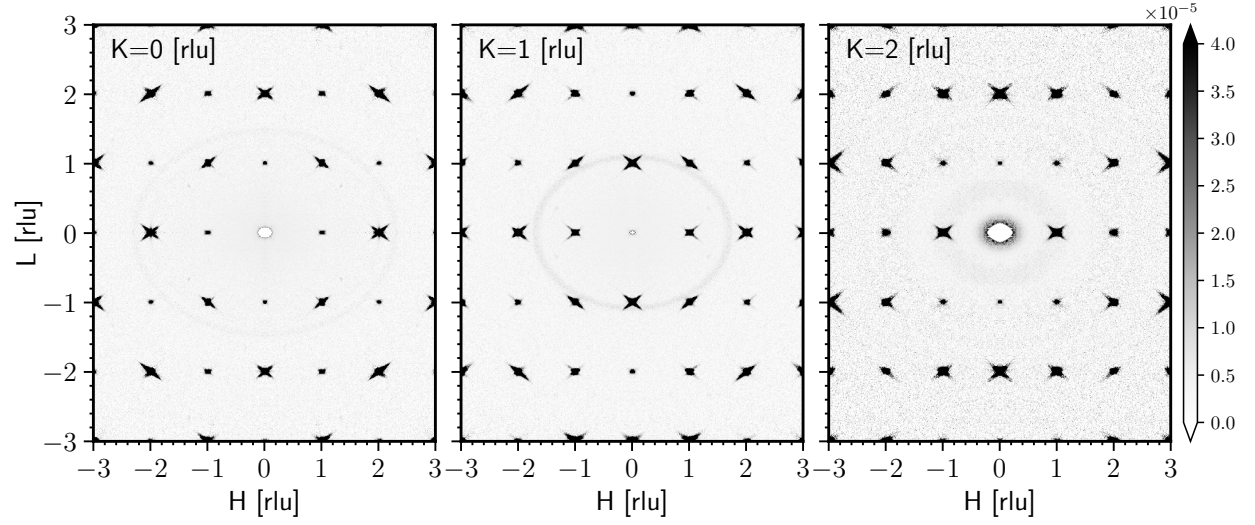

Fig. 29:  $Q$ -dependence, for integer  $K = 1$  rlu, of diffuse scattering from the ex-situ S1 dataset, with current along  $\mathbf{k}$ . The dark regions show pronounced diffuse scattering.

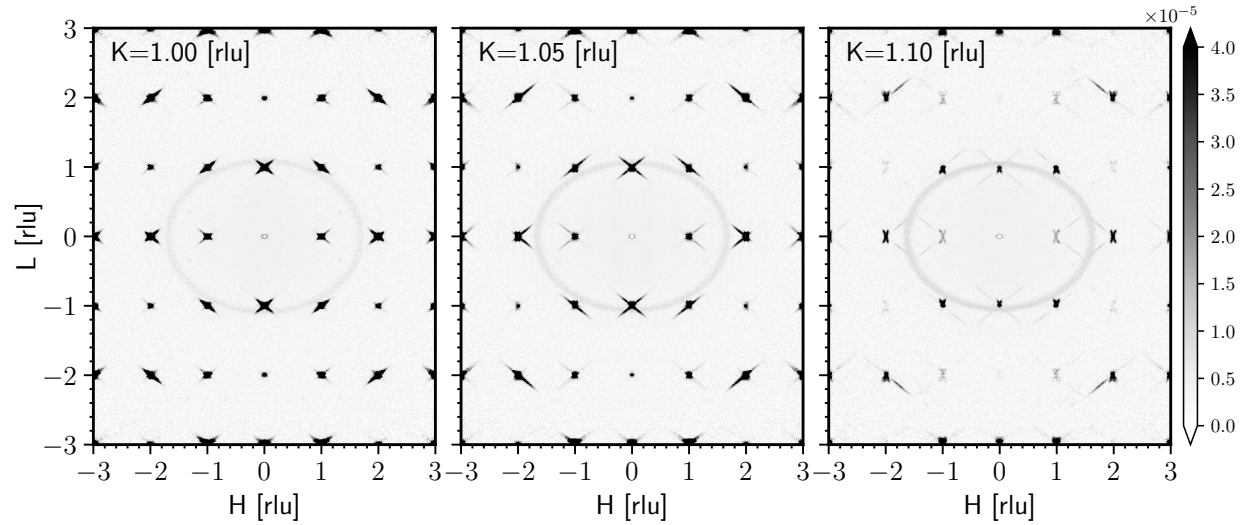

Fig. 30:  $Q$ -dependence near  $K = 1$  of diffuse scattering from the ex-situ S1 dataset, with current along  $\mathbf{k}$ . The dark regions show pronounced diffuse scattering.

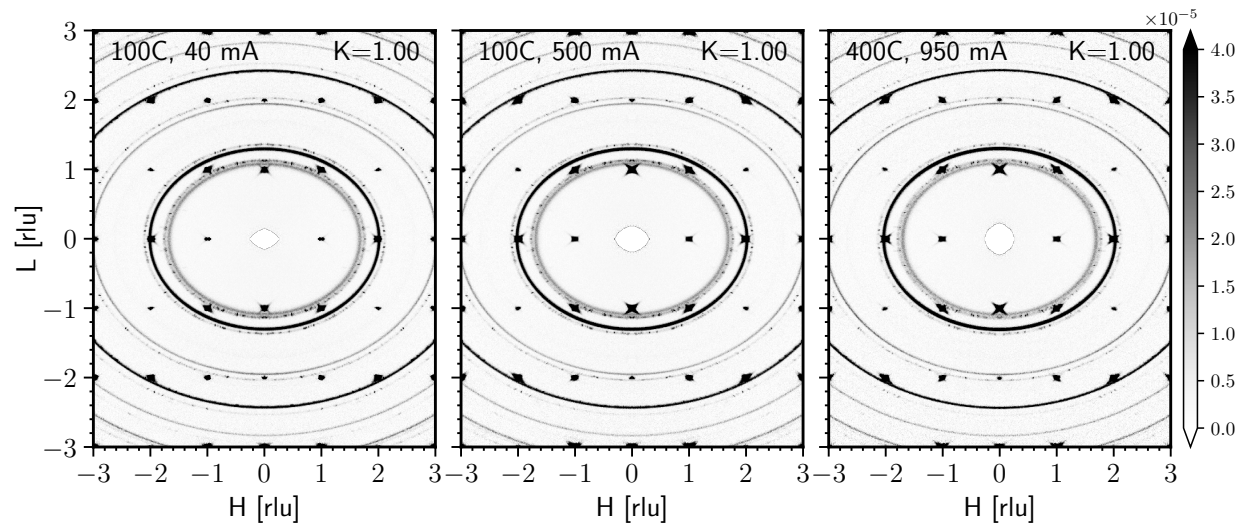

Fig. 31:  $Q$ -dependence near  $K = 1$  of diffuse scattering from the ex-situ S1 dataset, with current along  $\mathbf{k}$ . The dark regions show pronounced diffuse scattering.
